# Supplementary material for: Orthogonal series estimation of the pair correlation function of a spatial point process
Source: arXiv:1702.01736 source file (2017-02-06)
Supplement: Supplementary file 1 [file oseSupp.pdf]

# Supplementary material for 'Orthogonal series estimation of the pair correlation function of a spatial point process'

Abdollah Jalilian[1], Yongtao Guan[2], and Rasmus Waagepetersen[3]

[1]Department of Statistics, Razi University,Bagh-e-Abrisham, Kermanshah 67149-67346, Iran jalilian@razi.ac.ir
[2]Department of Management Science, University of Miami,Coral Gables, Florida 33124-6544, U.S.A. yguan@bus.miami.edu
[3]Department of Mathematical Sciences, Aalborg University,Fredrik Bajersvej 7G, DK-9220 Aalborg, Denmark rw@math.aau.dk

February 6, 2017

## S1 Expanding observation window

This section states a few results on the asymptotic behavior of the edge correction $e_n(h)$ (defined in (9) in the main document) and related ratios. For each $n \geq 1$ and $h, h_1, h_2 \in \mathbb{R}^d$,

$$|W_n \cap (W_n)_h| = \begin{cases} \prod_{i=1}^d (2na_i - |h_i|) & |h_i| < 2na_i, i = 1, \dots, d \\ 0 & \text{otherwise} \end{cases}$$

and

$$\left|W_n \cap (W_n)_{h_1} \cap (W_n)_{h_2}\right| = \begin{cases} V_n(h_1, h_2) & \max\{|h_{1i}|, |h_{2,i}|, |h_{1i} - h_{2i}|\} < 2na_i, i = 1, \dots, d \\ 0 & \text{otherwise} \end{cases}$$

where $V_n(h_1, h_2) = \prod_{i=1}^d \big(2na_i - \max\{0, h_{1i}, h_{2i}\} + \min\{0, h_{1i}, h_{2i}\}\big)$. Therefore, for any fixed $h, h_1, h_2 \in \mathbb{R}^d$, as $n \to \infty$,

$$e_n(h) = \frac{|W_n \cap (W_n)_h|}{|W_n|} = \prod_{i=1}^d \left(1 - \frac{|h_i|}{2na_i}\right) \to 1. \tag{1}$$

If $n \geq R/\min_{1 \leq i \leq d} a_i$ or equivalently $B_{r_{\min}}^R \subset W_n$, then $1/2^d \leq e_n(h) \leq 1$ for any $h \in B_{r_{\min}}^R$.

Further,

$$\frac{\left|W_n \cap (W_n)_{h_1} \cap (W_n)_{h_2}\right|}{|W_n|} = \prod_{i=1}^d \left(1 - \frac{\max\{0, h_{1i}, h_{2i}\} - \min\{0, h_{1i}, h_{2i}\}}{2na_i}\right) \to 1. \tag{2}$$

Similarly, it can be shown that for any fixed $h_1, h_2, h_3 \in \mathbb{R}^d$,

$$\left|W_n \cap (W_n)_{h_1} \cap (W_n)_{h_3} \cap (W_n)_{h_2 + h_3}\right| / |W_n| \to 1.$$

## S2 Mean and variance of $\hat{\theta}_{k,n}$

For $n$ large enough, $\mathbb{1}(h \in B_{r_{\min}}^R) > 0$ implies $|W_n \cap (W_n)_h| > 0$. Then, by the second order Campbell formula (see **?**, Section C.2.1),

$$\begin{aligned}
E(\hat{\theta}_{k,n}) =& \frac{1}{\text{sa}_d |W_n|} \int_{W_n^2} \mathbb{1}(v-u \in B_{r_{\min}}^R) \frac{\phi_k(\|v-u\| - r_{\min}) w(\|v-u\| - r_{\min})}{\|v-u\|^{d-1} e_n(v-u)} g(\|v-u\|) \mathrm{d}u \mathrm{d}v \\
=& \int_{\mathbb{R}^d} \mathbb{1}(h \in B_{r_{\min}}^R) \frac{g(\|h\|)\phi_k(\|h\| - r_{\min}) w(\|h\| - r_{\min})}{\text{sa}_d \|h\|^{d-1}} \int_{\mathbb{R}^d} \frac{\mathbb{1}\{v \in W_n \cap (W_n)_h\}}{|W_n \cap (W_n)_h|} \mathrm{d}v \mathrm{d}h \\
=& \int_{r_{\min}}^{r_{\min}+R} g(r)\phi_k(r - r_{\min}) w(r - r_{\min}) \mathrm{d}r = \theta_k.
\end{aligned}$$

Let $f_k(h) = \phi_k(\|h\| - r_{\min}) w(\|h\| - r_{\min}) / \|h\|^{d-1}$. Then, by the second to fourth order Campbell formulae (omitting the details),

$$\begin{aligned}
\text{var}(\hat{\theta}_{k,n}) = \frac{1}{(\text{sa}_d)^2 |W_n|} \Bigg[ & 2 \int_{B_{r_{\min}}^R} g(h) f_k^2(\|h\|) G_n^{(2)}(h) \mathrm{d}h \\
& + 4 \int_{B_{r_{\min}}^R} \int_{B_{r_{\min}}^R} g^{(3)}(h_1, h_2) f_k(\|h_1\|) f_k(\|h_2\|) G_n^{(3)}(h_1, h_2) \mathrm{d}h_1 \mathrm{d}h_2 \\
& + \int_{B_{r_{\min}}^R} \int_{B_{r_{\min}}^R} f_k(\|h_1\|) f_k(\|h_2\|) G_n^{(4)}(h_1, h_2) \mathrm{d}h_1 \mathrm{d}h_2 \Bigg], \qquad (3)
\end{aligned}$$

where

$$\begin{aligned}
G_n^{(2)}(h) &= \frac{1}{e_n^2(h)} \left[ \frac{1}{|W_n|} \int_{W_n} \frac{\mathbf{1}[u+h \in W_n]}{\rho(u)\rho(u+h)} \mathrm{d}u \right], \\
G_n^{(3)}(h_1, h_2) &= \frac{1}{e_n(h_1) e_n(h_2)} \left[ \frac{1}{|W_n|} \int_{W_n} \frac{\mathbf{1}[u \in (W_n)_{h_1} \cap (W_n)_{h_2}]}{\rho(u)} \mathrm{d}u \right], \\
G_n^{(4)}(h_1, h_2) &= \frac{1}{e_n(h_1) e_n(h_2)} \int_{\mathbb{R}^2} \left[ g^{(4)}(h_1, u, h_2 + u) - g(h_1) g(h_2) \right] \\
& \qquad \frac{\left| W_n \cap (W_n)_u \cap (W_n)_{h_1} \cap (W_n)_{h_2} \right|}{|W_n|} \mathrm{d}u.
\end{aligned}$$

For $n \geq R / \min_{1 \leq i \leq d} a_i$ and any $h, h_1, h_2 \in B_{r_{\min}}^R$, by V1,

$$\begin{aligned}
G_n^{(2)}(h) &= \frac{1}{e_n^2(h)} \left[ \frac{1}{|W_n|} \int_{W_n} \frac{\mathbf{1}[u+h \in W_n]}{\rho(u)\rho(u+h)} \mathrm{d}u \right] \leq \frac{1}{\rho_{\min}^2 e_n(h)} \leq \frac{2^d}{\rho_{\min}^2}, \\
G_n^{(3)}(h_1, h_2) &= \frac{1}{e_n(h_1) e_n(h_2)} \left[ \frac{1}{|W_n|} \int_{W_n} \frac{\mathbf{1}[u \in (W_n)_{h_1} \cap (W_n)_{h_2}]}{\rho(u)} \mathrm{d}u \right] \\
&\leq \frac{1}{\rho_{\min} e_n(h)} \leq \frac{2^d}{\rho_{\min}}
\end{aligned}$$

and by V3

$$\begin{aligned}
\left| G_n^{(4)}(h_1, h_2) \right| &\leq \frac{1}{e_n(h_1) e_n(h_2)} \int_{\mathbb{R}^2} \left| g^{(4)}(h_1, u, h_2 + u) - g(h_1) g(h_2) \right| \\
& \qquad \frac{\left| W_n \cap (W_n)_u \cap (W_n)_{h_1} \cap (W_n)_{h_2} \right|}{|W_n|} \mathrm{d}u \\
&\leq \frac{1}{e_n(h_1)} \int_{\mathbb{R}^2} \left| g^{(4)}(h_1, u, h_2 + u) - g(h_1) g(h_2) \right| \mathrm{d}u \\
&\leq 2^d \int_{\mathbb{R}^2} \left| g^{(4)}(h_1, u, h_2 + u) - g(h_1) g(h_2) \right| \mathrm{d}u \leq 2^d C_4.
\end{aligned}$$

Thus, using V2, for all $k \geq 1$ and $n \geq R/\min_{1\leq i\leq d} a_i$,

$$\mathrm{var}(\hat{\theta}_{k,n}) \leq \frac{1}{(\mathrm{sa}_d)^2|W_n|}\left[\frac{2^{d+1}}{\rho_{\min}^2}\int_{B_{r_{\min}}^R} f_k^2(\|h\|)g(\|h\|)\mathrm{d}h + \frac{2^{d+2}}{\rho_{\min}}C_3\left(\int_{B_{r_{\min}}^R}\big|f_k(\|h\|)\big|\mathrm{d}h\right)^2 + 2^dC_4\left(\int_{B_{r_{\min}}^R}\big|f_k(\|h\|)\big|\mathrm{d}h\right)^2\right].$$

But for all $k \geq 1$,

$$\begin{aligned}\int_{B_{r_{\min}}^R} f_k^2(\|h\|)g(\|h\|)\mathrm{d}h &= \int_{r_{\min}}^{r_{\min}+R}\phi_k^2(r-r_{\min})g(r)\frac{w^2(r-r_{\min})}{r^{d-1}}\mathrm{d}r\\ &= \int_0^R \phi_k^2(r)g(r+r_{\min})\frac{w^2(r)}{(r+r_{\min})^{d-1}}\mathrm{d}r\\ &\leq C_2\int_0^R\phi_k^2(r)w(r)\mathrm{d}r = C_2,\end{aligned}$$

and by Hölder's inequality,

$$\begin{aligned}\int_{B_{r_{\min}}^R}\big|f_k(\|h\|)\big|\mathrm{d}h &= \int_{B_{r_{\min}}^R}\big|\phi_k(\|h\|-r_{\min})\big|\frac{w(\|h\|-r_{\min})}{\|h\|^{d-1}}\mathrm{d}h\\ &= \int_{r_{\min}}^{r_{\min}+R}\big|\phi_k(r-r_{\min})\big|w(r-r_{\min})\mathrm{d}r\\ &\leq \left(\int_0^R\phi_k^2(r)w(r)\mathrm{d}r\right)^{1/2}\left(\int_0^R w(r)\mathrm{d}r\right)^{1/2} = \left(\int_0^R w(r)\mathrm{d}r\right)^{1/2} < \infty.\end{aligned}$$

Therefore

$$\mathrm{var}(\hat{\theta}_{k,n}) < \frac{1}{(\mathrm{sa}_d)^2|W_n|}\left[\frac{2^{d+1}}{\rho_{\min}^2}C_2 + \left(\frac{2^{d+2}}{\rho_{\min}}C_3 + 2^dC_4\right)\left(\int_0^R w(r)\mathrm{d}r\right)\right] = \frac{C_1}{|W_n|},$$

where

$$C_1 = \frac{1}{(\mathrm{sa}_d)^2}\left[\frac{2^{d+1}}{\rho_{\min}^2}C_2 + \left(\frac{2^{d+2}}{\rho_{\min}}C_3 + 2^dC_4\right)\left(\int_0^R w(r)\mathrm{d}r\right)\right] > 0.$$

# S3 Proof of asymptotic normality

In this section we give a proof of Theorem 1. Let for $\mathbf{t} = (t_1, \ldots, t_d) \in \mathbb{Z}^d$,

$$\Delta(\mathbf{t}) = \times_{i=1}^d\,(s(t_i - 1/2), s(t_i + 1/2)]$$

be the hyper-square with side length $s$ and centered at $s\mathbf{t}$. Then, $\{\Delta(\mathbf{t}) : \mathbf{t} \in \mathbb{Z}^d\}$ is a partition of $\mathbb{R}^d$; i.e., $\Delta(\mathbf{t}_1) \cap \Delta(\mathbf{t}_2) = \emptyset$ for $\mathbf{t}_1 \neq \mathbf{t}_2$ and $\cup_{\mathbf{t}\in\mathbb{Z}^d}\Delta(\mathbf{t}) = \mathbb{R}^d$, and $\big|\Delta_n(\mathbf{t}) \oplus R\big| = (s+2R)^d$, where

$$\Delta(\mathbf{t}) \oplus R = \times_{i=1}^d\,(s(t_i - 1/2) - R, s(t_i + 1/2) + R]\,.$$

Let $\mathcal{T}_n = \left\{\mathbf{t} \in \mathbb{Z}^d : \Delta(\mathbf{t}) \cap W_n \neq \emptyset\right\}$ and define

$$Y_n(\mathbf{t}) = \sum_{u\in X\cap\Delta(\mathbf{t})}\ \sum_{\substack{v\in X\backslash\{u\}\\ v-u\in B_{r_{\min}}^R}}\frac{f_n(v-u)\mathbb{1}(u\in W_n, v\in W_n)}{\rho(u)\rho(v)e_n(v-u)}.$$

Then, since $X = \bigcup_{\mathbf{t}\in\mathbb{Z}^d} \big(X \cap \Delta(\mathbf{t})\big)$,

$$
\begin{aligned}
S_n &= \frac{1}{\text{sa}_d|W_n|} \sum_{\substack{u,v\in X_{W_n}\\ v-u\in B^R_{r_{\min}}}}^{\neq} \frac{f_n(v-u)}{\rho(u)\rho(v)e_n(v-u)} \\
&= \frac{1}{\text{sa}_d|W_n|} \sum_{\mathbf{t}\in\mathbb{Z}^d} \sum_{u\in X\cap\Delta(\mathbf{t})} \sum_{\substack{v\in X\setminus\{u\}\\ v-u\in B^R_{r_{\min}}}} \frac{f_n(v-u)\mathbb{1}(u\in W_n, v\in W_n)}{\rho(u)\rho(v)e_n(v-u)} \\
&= \frac{1}{\text{sa}_d|W_n|} \sum_{\substack{\mathbf{t}\in\mathbb{Z}^d\\ \Delta(\mathbf{t})\cap W_n\neq\emptyset}} Y_n(\mathbf{t}) = \frac{1}{\text{sa}_d|W_n|} \sum_{\mathbf{t}\in\mathcal{T}_n} Y_n(\mathbf{t}).
\end{aligned}
$$

Due to V1, N4 and since $e_n(h) > 1/2^d$ for $n$ large enough and $h \in B^R_{r_{\min}}$,

$$
E(|Y_n(\mathbf{t})|^{2+\lceil\eta\rceil}) \le E\left( \sum_{u\in X\cap\Delta(\mathbf{t})} \sum_{\substack{v\in X\setminus\{u\}\\ v-u\in B^R_{r_{\min}}}} \frac{L_2 2^d}{\rho^2_{\min}} \right)^{2+\lceil\eta\rceil}.
$$

The moments $E(|Y_n(\mathbf{t})|^{2+\lceil\eta\rceil})$ are thus bounded by sums of integrals involving $g^{(k)}(u_1,\ldots,u_{k-1})$ times $(L_2 2^d/\rho^2_{\min})^{2+\lceil\eta\rceil}$ for $k = 2,\ldots,2(2+\lceil\eta\rceil)$. These integrals are bounded uniformly in $\mathbf{t}$ and $n$ due to assumption N2. Thus,

$$
\sup_{n\ge1}\sup_{\mathbf{t}\in\mathcal{T}_n} E(|Y_n(\mathbf{t})|^{2+\eta}) \le \sup_{n\ge1}\sup_{\mathbf{t}\in\mathcal{T}_n} E(|Y_n(\mathbf{t})|^{2+\lceil\eta\rceil}) < \infty
$$

and hence $\big\{|Y_n(\mathbf{t})|^{2+\eta} : \mathbf{t}\in\mathcal{T}_n, n\ge 1\big\}$ is a uniformly integrable family (triangular array) of random variables. Invoking finally N1 and N3 and letting $\sigma_n^2 = \text{var}\{\sum_{\mathbf{t}\in\mathcal{T}_n} Y_n(\mathbf{t})\}$, it follows directly from Theorem 3.1 in **?** that

$$
\sigma_n^{-1} \sum_{\mathbf{t}\in\mathcal{T}_n} \big[Y_n(\mathbf{t}) - E\{Y_n(\mathbf{t})\}\big] \xrightarrow{D} N(0,1),
$$

which is equivalent to Theorem 1.

# S4 Asymptotic mean of $\widehat{\theta^2_k}$

Consider a real function $f$ on $\mathbb{R}^d\times\mathbb{R}^d$ where $f(h_1,h_2)\neq 0$ implies $|W_n\cap(W_n)_{h_1}||W_n\cap(W_n)_{h_2}| > 0$. Then by the fourth order Campbell formula,

$$
\begin{aligned}
&E\left\{ \sum_{u,v,u',v'\in X_{W_n}}^{\neq} \frac{f(v-u,v'-u')}{\rho(u)\rho(v)\rho(u')\rho(v')|W_n\cap(W_n)_{v-u}||W_n\cap(W_n)_{v'-u'}|} \right\} \\
&= \int_{W_n^4} \frac{f(v-u,v'-u')}{|W_n\cap(W_n)_{v-u}||W_n\cap(W_n)_{v'-u'}|} g^{(4)}(v-u,u'-u,v'-u)\mathrm{d}u\mathrm{d}v\mathrm{d}u'\mathrm{d}v' \\
&= \int_{(\mathbb{R}^d)^4} f(h_1,h_2)g^{(4)}(h_1,u'-u,h_2+u'-u) \\
&\qquad \frac{\mathbb{1}\{u\in W_n\cap(W_n)_{h_1}, u'\in W_n\cap(W_n)_{h_2}\}}{|W_n\cap(W_n)_{h_1}||W_n\cap(W_n)_{h_2}|}\mathrm{d}u\mathrm{d}h_1\mathrm{d}u'\mathrm{d}h_2 \\
&= \int_{\mathbb{R}^d}\int_{\mathbb{R}^d} f(h_1,h_2)\left\{ \frac{\int_{W_n\cap(W_n)_{h_1}}\int_{W_n\cap(W_n)_{h_2}} g^{(4)}(h_1,u'-u,h_2+u'-u)\mathrm{d}u\mathrm{d}u'}{|W_n\cap(W_n)_{h_1}||W_n\cap(W_n)_{h_2}|} \right\}\mathrm{d}h_1\mathrm{d}h_2.
\end{aligned}
$$

This expectation is the sum of

$$A = \int_{\mathbb{R}^d}\int_{\mathbb{R}^d} f(h_1,h_2)\left\{\frac{\int_{W_n\cap(W_n)_{h_1}}\int_{W_n\cap(W_n)_{h_2}} g(h_1)g(h_2)}{|W_n\cap(W_n)_{h_1}||W_n\cap(W_n)_{h_2}|}\mathrm{d}u\mathrm{d}u'\right\}\mathrm{d}h_1\mathrm{d}h_2$$
$$= \int_{\mathbb{R}^d}\int_{\mathbb{R}^d} f(h_1,h_2)g(h_1)g(h_2)\mathrm{d}h_1\mathrm{d}h_2$$

and

$$B_n = \int_{\mathbb{R}^d}\int_{\mathbb{R}^d} f(h_1,h_2)$$
$$\left[\frac{\int_{W_n\cap(W_n)_{h_1}}\int_{W_n\cap(W_n)_{h_2}}\left\{g^{(4)}(h_1,u'-u,h_2+u'-u)-g(h_1)g(h_2)\right\}\mathrm{d}u\mathrm{d}u'}{|W_n\cap(W_n)_{h_1}||W_n\cap(W_n)_{h_2}|}\right]\mathrm{d}h_1\mathrm{d}h_2$$
$$= \int_{\mathbb{R}^d}\int_{\mathbb{R}^d} f(h_1,h_2)\Bigg[\int_{\mathbb{R}^d}\frac{|W_n\cap(W_n)_{h_1}\cap(W_n)_{h_3}\cap(W_n)_{h_2+h_3}|}{|W_n\cap(W_n)_{h_1}||W_n\cap(W_n)_{h_2}|}$$
$$\left\{g^{(4)}(h_1,h_3,h_2+h_3)-g(h_1)g(h_2)\right\}\mathrm{d}h_3\Bigg]\mathrm{d}h_1\mathrm{d}h_2.$$

We now specialize to $f(h_1,h_2) = f_k(h_1)f_k(h_2)$, where

$$f_k(h) = \phi_k(\|h\|-r_{\min})w(\|h\|-r_{\min})\mathbb{1}(h\in B^R_{r_{\min}})/(\mathrm{sa}_d\|h\|^{d-1}).$$

Then, by V3

$$|B_n| \le \int_{B^R_{r_{\min}}}\int_{B^R_{r_{\min}}} f_k(h_1)f_k(h_2)\Bigg[\int_{\mathbb{R}^d}\frac{|W_n\cap(W_n)_{h_1}\cap(W_n)_{h_3}\cap(W_n)_{h_2+h_3}|}{|W_n\cap(W_n)_{h_1}||W_n\cap(W_n)_{h_2}|}$$
$$\left|g^{(4)}(h_1,h_3,h_2+h_3)-g(h_1)g(h_2)\right|\mathrm{d}h_3\Bigg]\mathrm{d}h_1\mathrm{d}h_2$$
$$\le C_4\int_{B^R_{r_{\min}}}\int_{B^R_{r_{\min}}}\frac{f_k(h_1)f_k(h_2)}{|W_n\cap(W_n)_{h_1}|}\mathrm{d}h_1\mathrm{d}h_2.$$

Thus $B_n$ tends to zero as $n\to\infty$. Regarding $A$, we have

$$A = \int_{\mathbb{R}^d}\int_{\mathbb{R}^d} f_k(h_1)f_k(h_2)g(h_1)g(h_2)\mathrm{d}h_1\mathrm{d}h_2 = \left\{\int_{\mathbb{R}^d} f_k(h)g(h)\mathrm{d}h\right\}^2$$
$$= \left\{\int_{r_{\min}}^{r_{\min}+R} g(r)\phi_k(r-r_{\min})w(r-r_{\min})\mathrm{d}r\right\}^2 = \theta_k^2.$$

# S5 Asymptotic behavior of Bessel function roots

It is known (see **?**, p. 199) that as $r\to\infty$,

$$J_\nu(r)\sim\left(\frac{2}{\pi r}\right)^{1/2}\cos\left(r-\frac{\nu\pi}{2}-\frac{\pi}{4}\right),$$

which implies that

$$\alpha_{\nu,k} = (k+\frac{\nu}{2}-\frac{1}{4})\pi + O(k^{-1}),\quad \text{as } k\to\infty, \tag{4}$$

and $\alpha_{\nu,k}\to\infty$, as $k\to\infty$. We can argue that for large $k$,

$$J_{\nu+1}(\alpha_{\nu,k}) \approx \left(\frac{2}{\pi\alpha_{\nu,k}}\right)^{1/2}\cos\left(\alpha_{\nu,k}-\frac{\pi}{4}-\frac{(\nu+1)\pi}{2}\right)$$
$$= \left(\frac{2}{\pi\alpha_{\nu,k}}\right)^{1/2}\cos\left((k-1)\pi+O(k^{-1})\right),$$

and consequently

$$\big|J_{\nu+1}(\alpha_{\nu,k})\big| \approx \left(\frac{2}{\pi\alpha_{\nu,k}}\right)^{1/2}. \tag{5}$$

# S6 Order of sum of products of Bessel basis functions

In this section we consider the Bessel basis in the case $r_{\min} = 0$. For $\nu \geq 0$ and $r > 0$ (?),

$$\big|J_\nu(r)\big| \leq \frac{c}{|r|^{1/3}},$$

where $c = 0.7857468704\ldots$, and hence

$$\big|\phi_k(r)\big| \leq \frac{cr^{-\nu-1/3}\sqrt{2}}{(R^2\alpha_{\nu,k})^{1/3}\big|J_{\nu+1}(\alpha_{\nu,k})\big|} \quad r > 0, k \geq 1.$$

Using (4) and (5), for large $k$,

$$\frac{cr^{-\nu-1/3}\sqrt{2}}{(R^2\alpha_{\nu,k})^{1/3}\big|J_{\nu+1}(\alpha_{\nu,k})\big|} \approx c\sqrt{\pi}\frac{r^{-\nu-1/3}}{R^{2/3}}\alpha_{\nu,k}^{1/6} \approx c\sqrt{\pi}\frac{r^{-\nu-1/3}}{R^{2/3}}\{(k+\frac{\nu}{2}-\frac{1}{4})\pi\}^{1/6}.$$

Since $\lim_{r\to 0} J_\nu(r)r^{-\nu} = \{\Gamma(\nu+1)2^\nu\}^{-1}$, we also obtain for large $k$ and $0 < \|h\| < R$,

$$|\phi(\|h\|)| \leq \text{const}\left(\frac{R}{\alpha_{\nu,k}}\right)^{-\nu}\frac{\sqrt{2}}{RJ_{\nu+1}(\alpha_{\nu,k})} \approx \text{const}\sqrt{\pi}\frac{\alpha_{\nu,k}^{\nu+1/2}}{R^{\nu+1}} = O(k^{\nu+1/2}).$$

Thus, for fixed $r$ and $0 < \|h\| < R$,

$$|\phi_k(r)\phi_k(\|h\|)| = O(k^{1/6+\max(1/6,\nu+1/2)}) = O(k^{1/6+\max(1/6,d/2-1/2)}).$$

By generalization of Faulhaber's formula (?),

$$\sum_{k=1}^{K_n} k^p = O(K_n^{p+1}), \quad p > -1.$$

Therefore,

$$\frac{1}{K_n^\omega}\sum_{k=1}^{K_n}\big|\phi_k(r)\phi_k(\|h\|)\big| = \begin{cases} O(K_n^{4/3-\omega}) & d = 1 \\ O(K_n^{d/2+2/3-\omega}) & d > 1 \end{cases}$$

for $\omega > 0$ and $0 < r, \|h\| < R$.

# S7 Simulation study

The results in Figure S1 are obtained as for the simulation study in the main document but with $W = [0,2]^2$. The estimated cut-offs $\hat{K}$ are summarized in Table S1. Simulation mean and 95% envelopes for $\hat{g}_k$, $\hat{g}_c$ and $\hat{g}_o$ with both Fourier-Bessel and cosine basis and simple smoothing schemes are shown in Figure S2 and Figure S3. Figure S4 shows histograms of orthogonal series estimates. Comments on these figures and the table are given in the main document.

# S8 Data example

Figure S5 shows the data sets and fitted intensity functions considered in Section 7 of the main document. For the *Capparis frondosa* species and the orthogonal series estimator with cosine basis, the function $\hat{I}(K)$ given in (14) of the main document is shown in Figure S6. Although $\hat{I}(K)$ is decreasing over $1 \leq K \leq 49$, the rate of decrease slows down after $K = 7$.

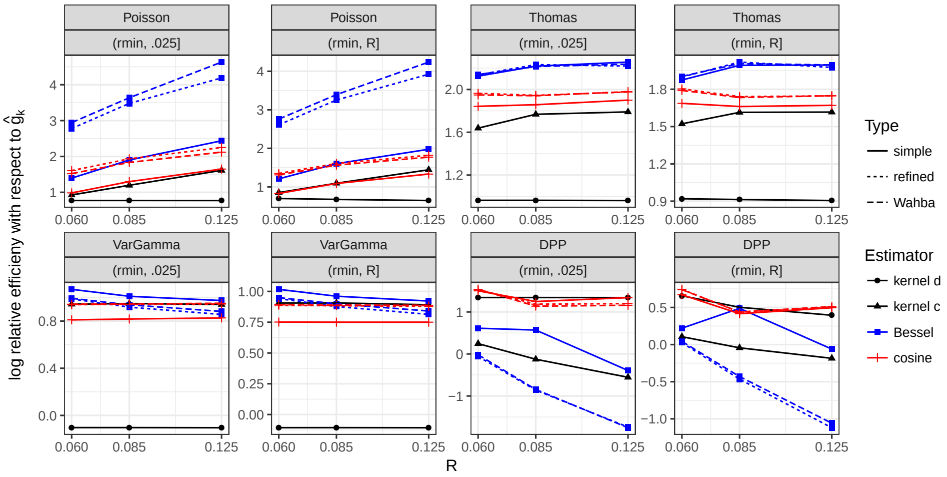


Figure S1: Plots of log relative efficiencies for small lags $(r_{\min}, 0.025]$ and all lags $(r_{\min}, R]$, $R = 0.06, 0.085, 0.125$, and $W = [0,2]^2$. Black: kernel estimators. Blue and red: orthogonal series estimators with Bessel respectively cosine basis. Lines serve to ease visual interpretation.

Table S1: Carlo mean and quantiles of the estimated cut-off $\hat{K}$ obtained from (15) for the orthogonal series estimator with Bessel ($\hat{g}_{o1}$) and cosine ($\hat{g}_{o4}$) basis in the case of Poisson (P), Thomas (T), Variance Gamma (V) and determinantal (D) point processes on observation windows $W_1 = [0,1]^2$ and $W_2 = [0,2]^2$ with $r_{\min} = 0.001$.

| | | | $R = 0.06$ | | | $R = 0.085$ | | | $R = 0.125$ | | |
|---|---|---|---|---|---|---|---|---|---|---|---|
| | | | $\hat{E}(\hat{K})$ | $\hat{q}_{0.05}(\hat{K})$ | $\hat{q}_{0.95}(\hat{K})$ | $\hat{E}(\hat{K})$ | $\hat{q}_{0.05}(\hat{K})$ | $\hat{q}_{0.95}(\hat{K})$ | $\hat{E}(\hat{K})$ | $\hat{q}_{0.05}(\hat{K})$ | $\hat{q}_{0.95}(\hat{K})$ |
| $W_1$ | P | $\hat{g}_{o1}$ | 2.17 | 2.00 | 3.00 | 2.15 | 2.00 | 3.00 | 2.11 | 2.00 | 3.00 |
| $W_1$ | P | $\hat{g}_{o4}$ | 2.17 | 2.00 | 4.00 | 2.15 | 2.00 | 4.00 | 2.11 | 2.00 | 4.00 |
| $W_1$ | T | $\hat{g}_{o1}$ | 2.24 | 2.00 | 3.00 | 2.24 | 2.00 | 3.00 | 3.23 | 2.00 | 4.05 |
| $W_1$ | T | $\hat{g}_{o4}$ | 2.24 | 2.00 | 4.00 | 2.24 | 2.00 | 4.00 | 3.23 | 3.00 | 5.00 |
| $W_1$ | V | $\hat{g}_{o1}$ | 2.77 | 2.00 | 4.00 | 3.50 | 2.00 | 6.00 | 4.85 | 3.00 | 8.00 |
| $W_1$ | V | $\hat{g}_{o4}$ | 2.77 | 2.00 | 5.00 | 3.50 | 2.00 | 7.00 | 4.85 | 3.00 | 10.00 |
| $W_1$ | D | $\hat{g}_{o1}$ | 2.21 | 2.00 | 3.00 | 2.18 | 2.00 | 3.00 | 2.38 | 2.00 | 3.00 |
| $W_1$ | D | $\hat{g}_{o4}$ | 2.21 | 2.00 | 3.00 | 2.18 | 2.00 | 4.00 | 2.38 | 2.00 | 5.00 |
| $W_2$ | P | $\hat{g}_{o1}$ | 2.17 | 2.00 | 3.00 | 2.12 | 2.00 | 3.00 | 2.09 | 2.00 | 3.00 |
| $W_2$ | P | $\hat{g}_{o4}$ | 2.17 | 2.00 | 4.00 | 2.12 | 2.00 | 4.00 | 2.09 | 2.00 | 4.00 |
| $W_2$ | T | $\hat{g}_{o1}$ | 2.39 | 2.00 | 4.00 | 2.46 | 2.00 | 4.00 | 3.78 | 3.00 | 5.00 |
| $W_2$ | T | $\hat{g}_{o4}$ | 2.39 | 2.00 | 5.00 | 2.46 | 2.00 | 5.00 | 3.78 | 3.00 | 6.00 |
| $W_2$ | V | $\hat{g}_{o1}$ | 3.58 | 3.00 | 5.00 | 5.14 | 3.00 | 8.00 | 7.19 | 5.00 | 11.00 |
| $W_2$ | V | $\hat{g}_{o4}$ | 3.58 | 3.00 | 9.00 | 5.14 | 4.00 | 12.00 | 7.19 | 5.00 | 17.00 |
| $W_2$ | D | $\hat{g}_{o1}$ | 2.22 | 2.00 | 4.00 | 2.17 | 2.00 | 3.00 | 2.79 | 2.00 | 4.00 |
| $W_2$ | D | $\hat{g}_{o4}$ | 2.22 | 2.00 | 3.00 | 2.17 | 2.00 | 4.00 | 2.79 | 3.00 | 5.00 |

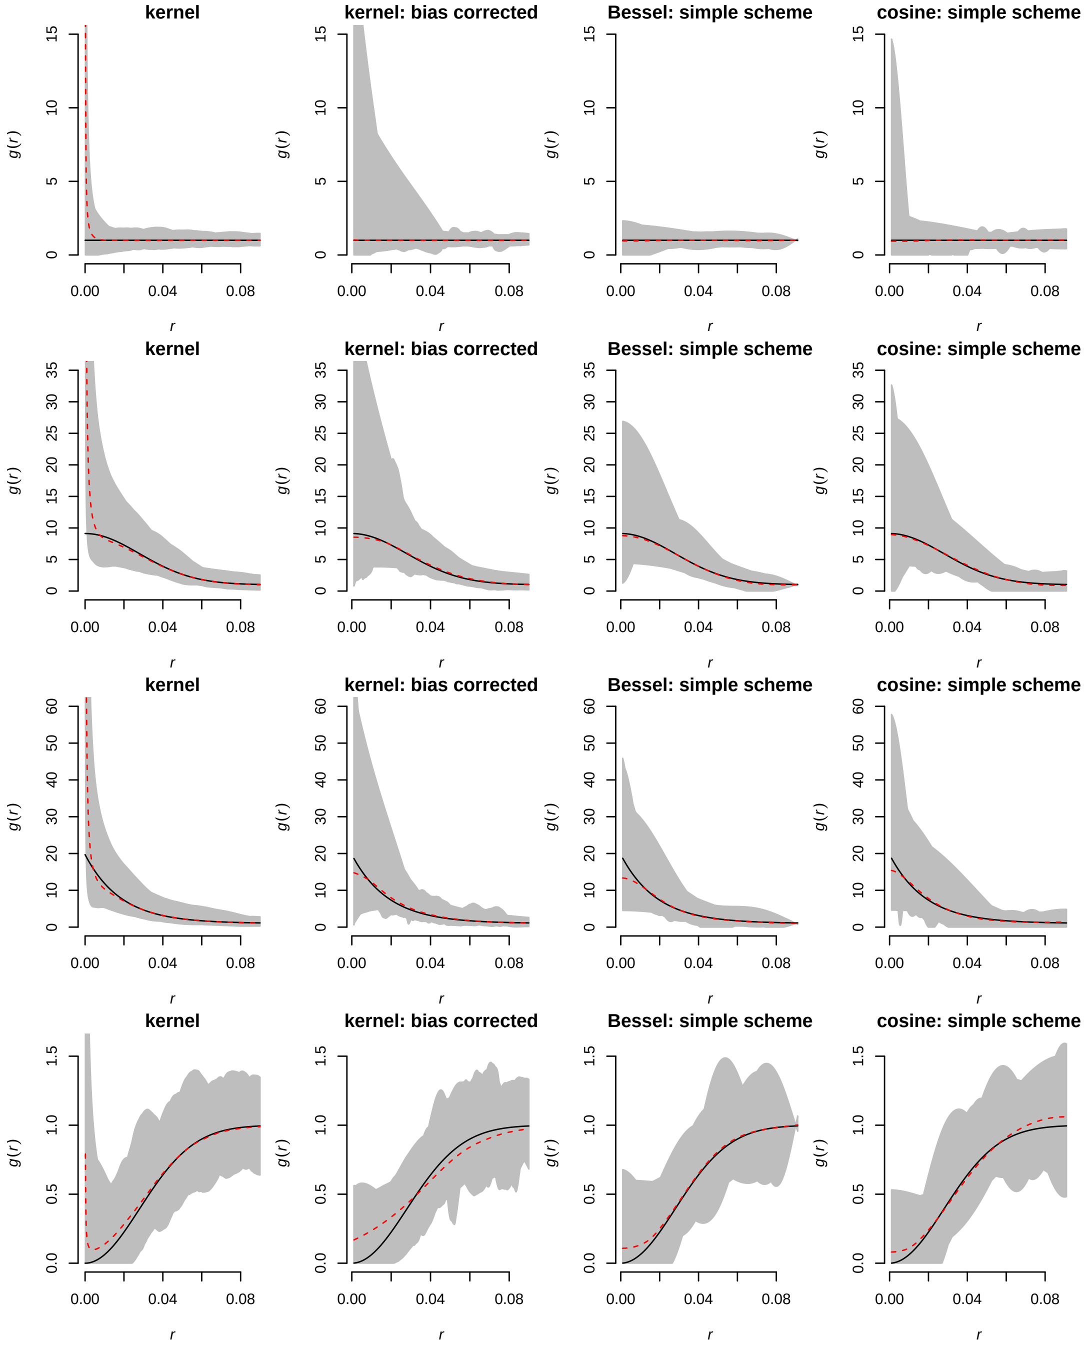


Figure S2: True pair correlation function (solid line), Monte Carlo mean (dashed lines) and 95% pointwise probability interval (grey area) of estimates based on $n_{\text{sim}} = 1000$ simulations from the Poisson (first row), Thomas (second row), Variance Gamma (third row) and determinantal (fourth row) point processes on $W = [0, 1]^2$.

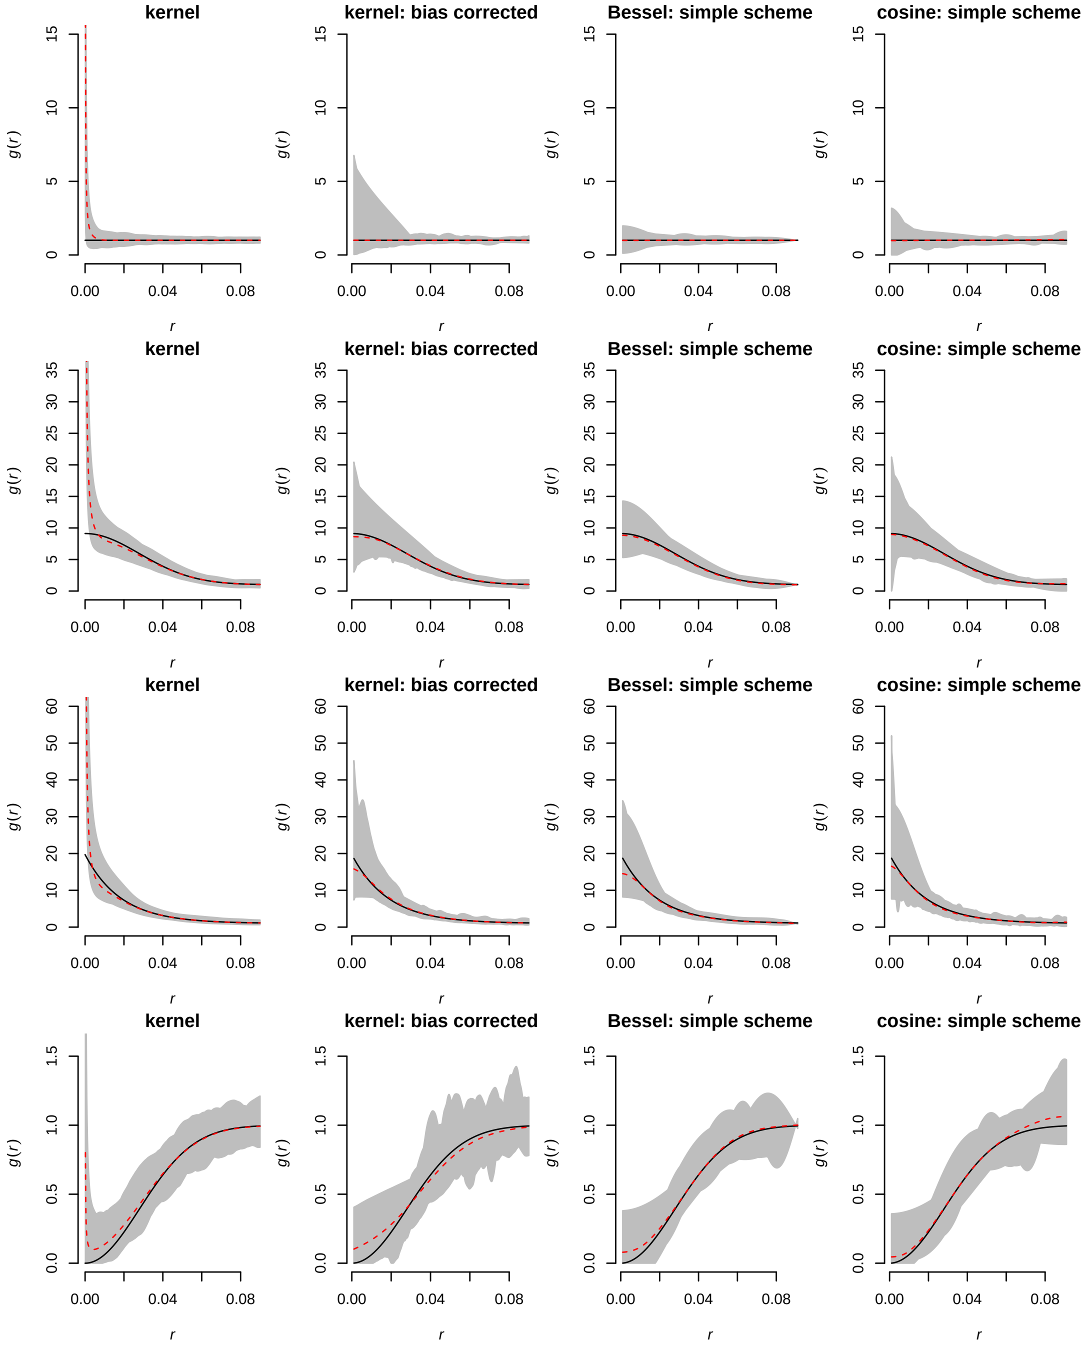


Figure S3: True pair correlation function (solid line), Monte Carlo mean (dashed lines) and 95% pointwise probability interval (grey area) of estimates based on $n_{\text{sim}} = 1000$ simulations from the Poisson (first row), Thomas (second row), Variance Gamma (third row) and determinantal (fourth row) point processes on $W = [0, 2]^2$.

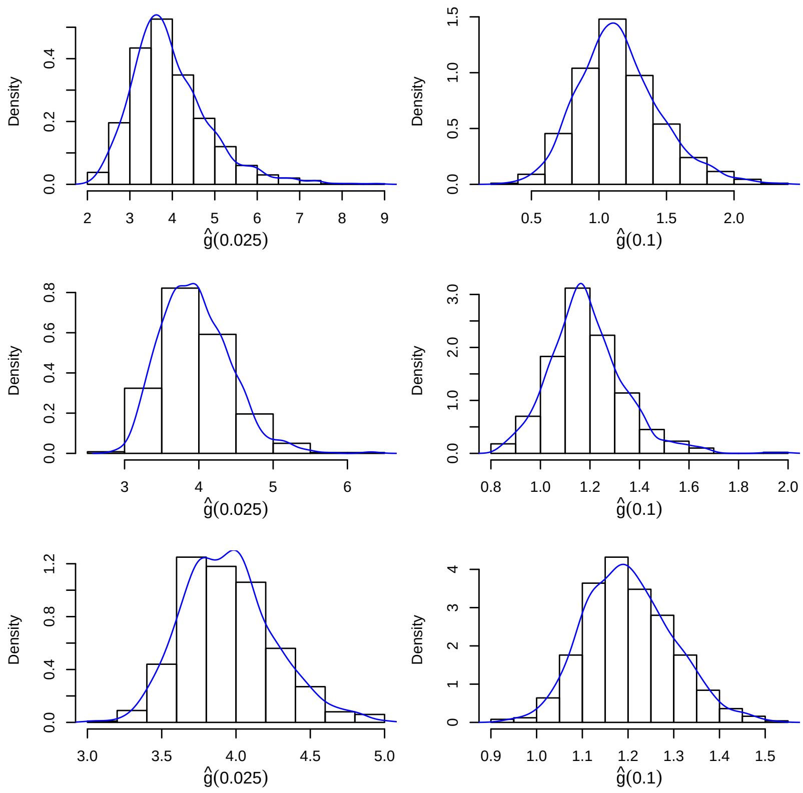


Figure S4: Histograms of $\hat{g}_o(r)$ at $r = 0.025$ and $r = 0.1$ using the Bessel basis with the simple smoothing scheme in case of the Thomas process on $W = [0,1]^2$ (upper panels), $W = [0,2]^2$ (middle panels) and $W = [0,3]^2$ (lower panels).

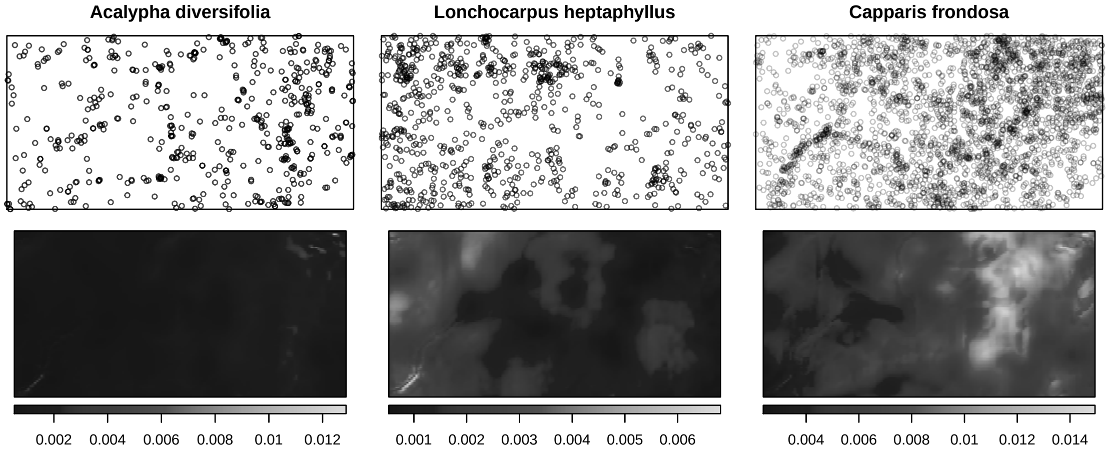


Figure S5: Locations of *Acalypha diversifolia*, *Lonchocarpus heptaphyllus* and *Capparis frondosa* trees in the Barro Colorado Island plot (upper panels) and their fitted parametric intensity functions (lower panels).

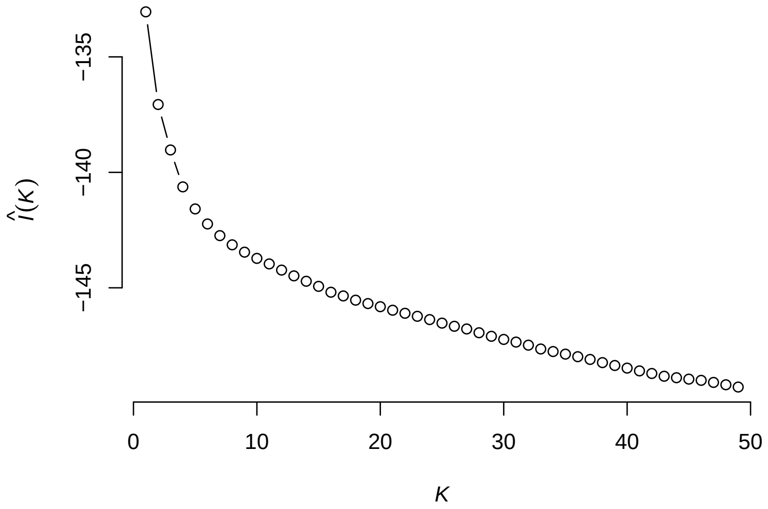


Figure S6: Estimate $\hat{I}(K)$ of the mean integrated squared error for *Capparis frondosa* in case of the orthogonal series estimator with cosine basis.

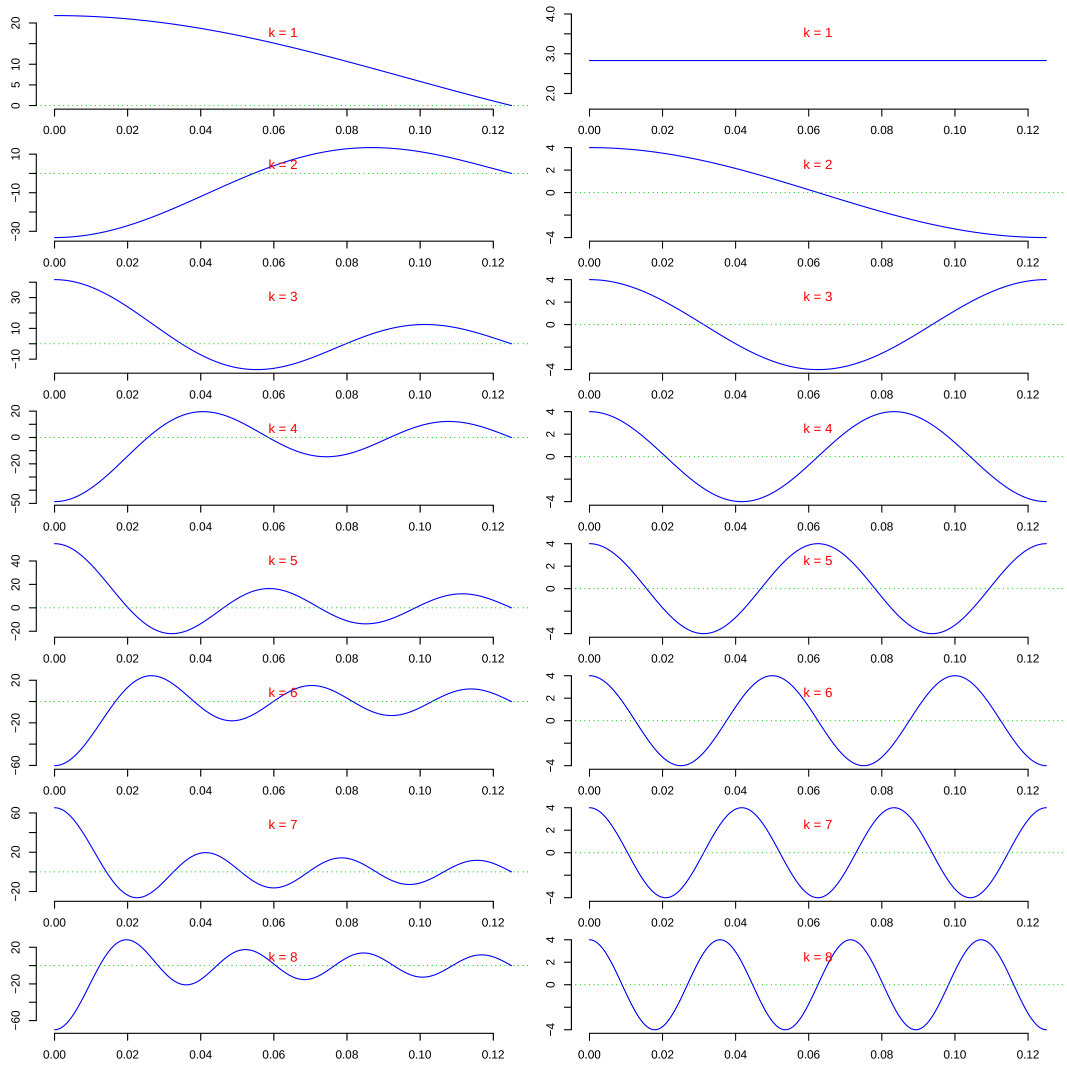


Figure S7: Fourier-Bessel and cosine basis functions $\phi_k(r)$ in the planar case ($d = 2$) for $R = 0.125$ and $k = 1, \ldots, 8$.

## S9 Behavior of the Fourier-Bessel and cosine basis

Figure S7 shows the Fourier-Bessel and cosine basis functions $\phi_k(r)$ in the planar case ($d = 2$) for $R = 0.125$, $k = 1, \dots, 8$ and $r \in [0, 0.125]$. Obviously, the cosine basis functions are uniformly bounded and integrable. However, the Fourier-Bessel basis functions exhibit damped oscillation behavior with $\phi_k(R) = 0$ and

$$\phi_k(0) = \frac{\alpha_{\nu,k}^{\nu}}{R^{\nu+1}2^{\nu-1/2}\Gamma(\nu+1)J_{\nu+1}(\alpha_{\nu,k})},$$

for all $k \geq 1$, because $\lim_{r\to 0} J_\nu(r)r^{-\nu} = 1/(\Gamma(\nu+1)2^\nu)$ for $\nu \geq 0$. Thus, $\phi_k(0) \to \infty$ as $k \to \infty$.

For $0 \leq \nu \leq 1/2$ (or equivalently $d = 2, 3$), $|J_\nu(r)| \leq (2/\pi r)^{1/2}$ and hence

$$\int_0^{\alpha_{\nu,k}} \big|J_\nu(r)\big| r^{\nu+1}\mathrm{d}r \leq \left(\frac{2}{\pi}\right)^{1/2} \int_0^{\alpha_{\nu,k}} r^{\nu+\frac{1}{2}}\mathrm{d}r = \left(\frac{2}{\pi}\right)^{1/2} \frac{(\alpha_{\nu,k})^{\nu+\frac{3}{2}}}{\nu+\frac{3}{2}}.$$

Therefore, as $k \to \infty$,

$$\begin{aligned}
\int_0^R \big|\phi_k(r)\big| w(r)\mathrm{d}r &= \frac{\sqrt{2}}{R\big|J_{\nu+1}(\alpha_{\nu,k})\big|}\left(\frac{R}{\alpha_{\nu,k}}\right)^{\nu+2} \int_0^{\alpha_{\nu,k}} \big|J_\nu(r)\big| r^{\nu+1}\mathrm{d}r \\
&\leq \frac{\sqrt{2}}{R\big|J_{\nu+1}(\alpha_{\nu,k})\big|}\left(\frac{R}{\alpha_{\nu,k}}\right)^{\nu+2} \left(\frac{2}{\pi}\right)^{1/2} \frac{(\alpha_{\nu,k})^{\nu+\frac{3}{2}}}{\nu+\frac{3}{2}} \\
&= \frac{2R^{\nu+1}}{\big|J_{\nu+1}(\alpha_{\nu,k})\big|(\pi\alpha_{\nu,k})^{1/2}(\nu+\frac{3}{2})} \\
&\approx \frac{2R^{\nu+1}}{(\frac{2}{\pi\alpha_{\nu,k}})^{1/2}(\pi\alpha_{\nu,k})^{1/2}(\nu+\frac{3}{2})} = \frac{\sqrt{2}R^{\nu+1}}{\nu+\frac{3}{2}} < \infty,
\end{aligned}$$

which implies uniform integrability of $\phi_k(r)$.
